# Supplementary material for: SHAP@k:Efficient and Probably Approximately Correct (PAC) Identification of Top-k Features
Source: arXiv:2307.04850 source file (2023-07-10)
Supplement: Supplementary file 1 [file 8.appendix.tex]

\section{Appendix}
